# Supplementary material for: Refined Catalan and Narayana cyclic sieving
Source: arXiv:2010.11157 source file (2020-11-04)

|   |   |   |
|---|---|---|
| 1 | 2 | 3 |
| 4 | 5 | 6 |

|   |   |   |
|---|---|---|
| 1 | 2 | 4 |
| 3 | 5 | 6 |

|   |   |   |
|---|---|---|
| 1 | 2 | 5 |
| 3 | 4 | 6 |

|   |   |   |
|---|---|---|
| 1 | 3 | 4 |
| 2 | 5 | 6 |

|   |   |   |
|---|---|---|
| 1 | 3 | 5 |
| 2 | 4 | 6 |

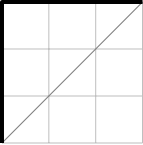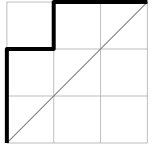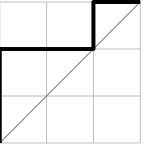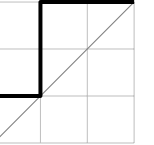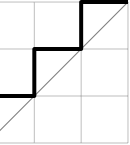

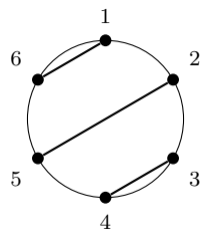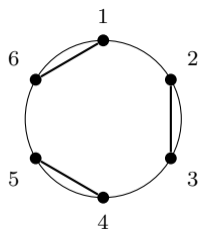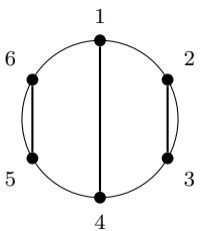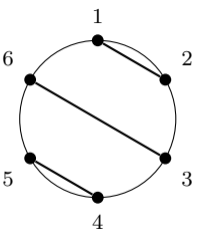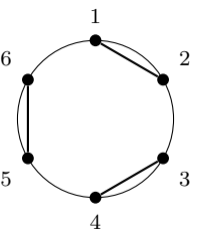

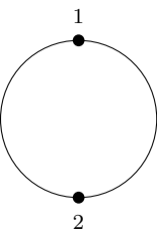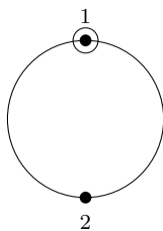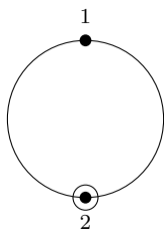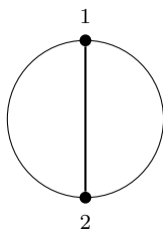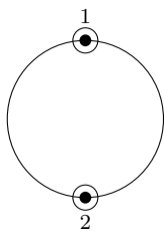

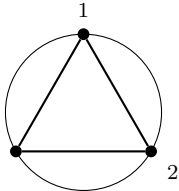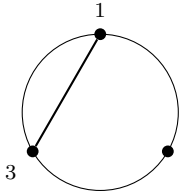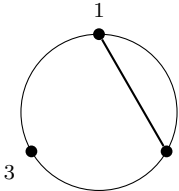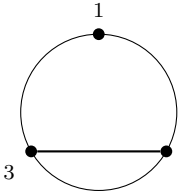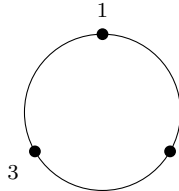

$\emptyset$

|   |   |
|---|---|
| 2 | 2 |
|---|---|

|   |   |
|---|---|
| 1 | 2 |
|---|---|

|   |   |
|---|---|
| 1 | 1 |
|---|---|

|   |   |
|---|---|
| 1 | 1 |
| 2 | 2 |

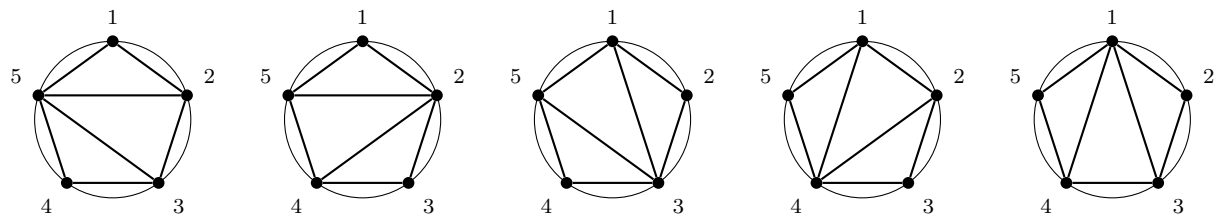

Supplement: Supplementary file 1 [file appendixAFigures.pdf]
