# Supplementary material for: Refined Catalan and Narayana cyclic sieving
Source: arXiv:2010.11157 source file (2020-11-04)

|   |   |   |   |
|---|---|---|---|
|   |   | 1 | 2 |
| 3 | 4 |   |   |

|   |   |   |   |
|---|---|---|---|
|   |   | 1 | 3 |
| 2 | 4 |   |   |

|   |   |   |   |
|---|---|---|---|
|   |   | 1 | 4 |
| 2 | 3 |   |   |

|   |   |   |   |
|---|---|---|---|
|   |   | 2 | 3 |
| 1 | 4 |   |   |

|   |   |   |   |
|---|---|---|---|
|   |   | 2 | 4 |
| 1 | 3 |   |   |

|   |   |   |   |
|---|---|---|---|
|   |   | 3 | 4 |
| 1 | 2 |   |   |

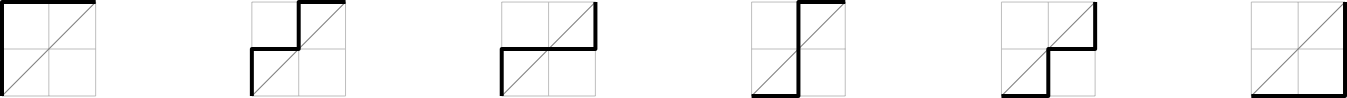

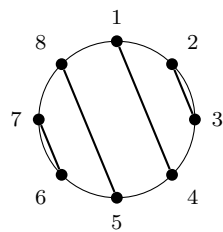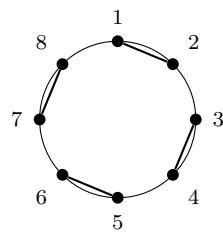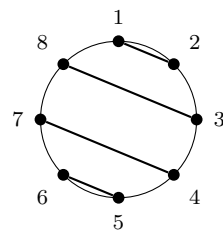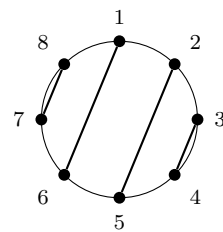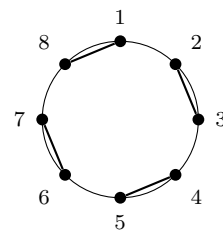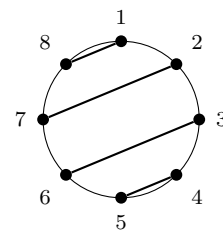

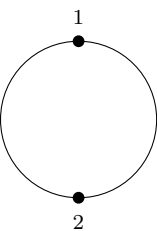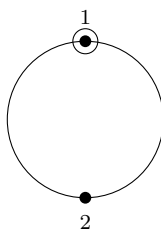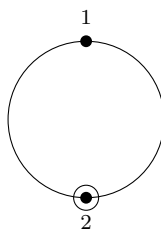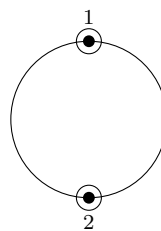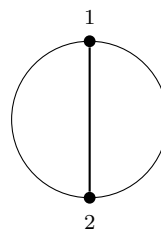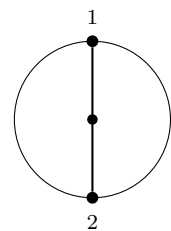

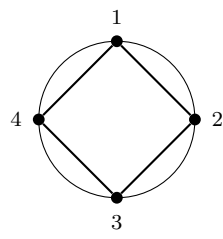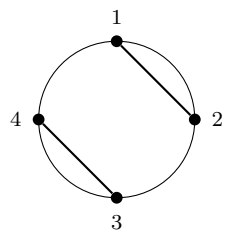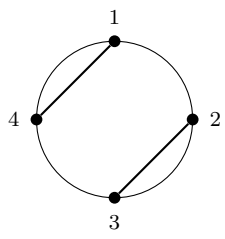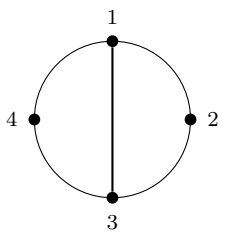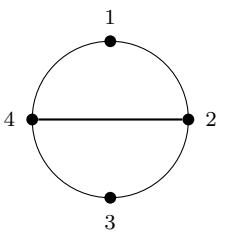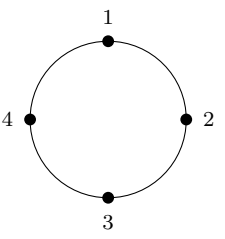

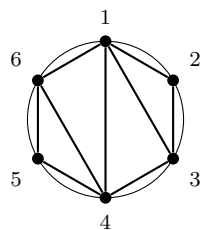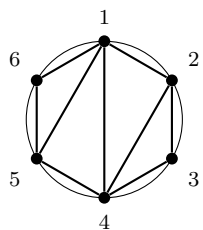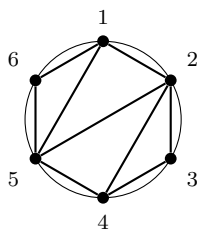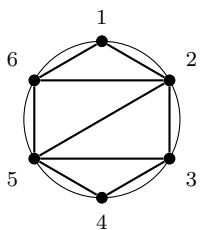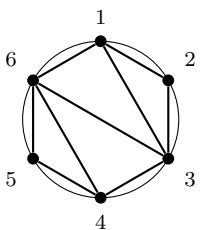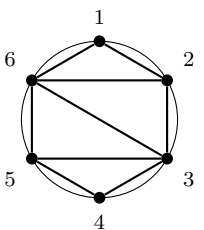

Supplement: Supplementary file 2 [file appendixBFigures.pdf]
